# Supplementary material for: Optimizing Parameters for Static Equilibrium of Discrete Elastic Rods with Active-Set Cholesky
Source: arXiv:2412.16461 source file (2025-10-14)
Supplement: Supplementary file 1 [file 8_appendix.tex]

\appendices

%%%%%%%%%%%%%%%%%%%%%%%%%%%%%%%%%%%%%%%%%%%%%%%%%%%%%%%%%%%%%%%%%%%%%%%%%%%%%%%
%%%%%%%%%%%%%%%%%%%%%%%%%%%%%%%%%%%%%%%%%%%%%%%%%%%%%%%%%%%%%%%%%%%%%%%%%%%%%%%

\section{Details on Gradient}
\label{sec:details_on_gradient}
In the following, we provide details on the gradient of the objectives. The gradient of the inertia objective is given by
\begin{align}
\nabla E_{\mathrm{in}}(\generalizedPos) = 
\frac{\generalizedMass}{\dt^2}(\generalizedPos - \generalizedPos^*).
\label{eq:inertia_gradient}
\end{align}
The gradient of the stretching objective on edge $i$ is given by
\begin{align}
\nabla_{\vertexPos_{i+1}} 
E_{\mathrm{st}, i}(\vertexPos_{i}, \vertexPos_{i+1}) 
&= -
\nabla_{\vertexPos_{i}} 
E_{\mathrm{st}, i}(\vertexPos_{i}, \vertexPos_{i+1})
\\
&= \stiffnessScale \stretchCoef_i \pi \radius^2 (\length_i \restLength_i^{-1} - 1) \tangent_i,
\label{eq:stretch_grad}
\end{align}
where $\tangent_i = \frac{\vertexPos_{i+1} - \vertexPos_{i}}{\length_i}$ denotes the unit tangent vector of edge $i$. Following \cite{Takahashi2025rest}, the 11-dimensional gradient of the bending objective on vertex $i$ is given by 
\begin{align}
\nabla E_{\mathrm{be}, i}(\yvec_i) = 
\left(\frac{\stiffnessScale \bendCoef_i \pi \radius^4}{4 (\restLength_{i-1} + \restLength_{i})}\right)
\Jacobian_{\mathrm{cu}, i}^T (\curvature_i - \restCurvature_i),
\label{eq:bending_i_grad}
\end{align}
where $\Jacobian_{\mathrm{cu}, i} \in \realNumber^{4 \times 11}$ denotes the Jacobian of $\curvature_i$ with respect to $\yvec_i$. Here, $\Jacobian_{\mathrm{cu}, i}^T (\curvature_i - \restCurvature_i) = \sum_{j=0}^3(\curvature_{i, j} - \restCurvature_{i, j})\nabla \curvature_{i, j}$, where $\curvature_{i, j}$ denotes the $j$th entry of $\curvature_i$ \mycolor{\cite{Panetta2019,Fei2019}}. Similarly, the 11-dimensional gradient of the twisting objective is given by
\begin{align}
\nabla E_{\mathrm{tw}, i}(\yvec_i) = 
\left(\frac{\stiffnessScale \twistCoef_i \pi \radius^4}{(\restLength_{i-1} + \restLength_{i})}\right)
(\twist_i - \restTwist_i) \nabla \twist_i.
\label{eq:twist_i_grad}
\end{align}

%%%%%%%%%%%%%%%%%%%%%%%%%%%%%%%%%%%%%%%%%%%%%%%%%%%%%%%%%%%%%%%%%%%%%%%%%%%%%%%
%%%%%%%%%%%%%%%%%%%%%%%%%%%%%%%%%%%%%%%%%%%%%%%%%%%%%%%%%%%%%%%%%%%%%%%%%%%%%%%

\section{Forces and Jacobians}
\label{sec:jacobian}

%%%%%%%%%%%%%%%%%%%%%%%%%%%%%%%%%%%%%%%%%%%%%%%%%%%%%%%%%%%%%%%%%%%%%%%%%%%%%%%
%%%%%%%%%%%%%%%%%%%%%%%%%%%%%%%%%%%%%%%%%%%%%%%%%%%%%%%%%%%%%%%%%%%%%%%%%%%%%%%

\subsection{Inertia}
Given the inertia force defined as $\generalizedForce_{\mathrm{in}} = -
\nabla E_{\mathrm{in}}(\generalizedPos)$ with $\generalizedPos = \generalizedPos^t$ and $\generalizedVel^t = 0$ for a static equilibrium case, we have
$\generalizedForce_{\mathrm{in}} = \generalizedForceExt$ and thus $\frac{\partial \generalizedForce_{\mathrm{in}}}
{\partial \parameter} = 0$ \cite{Takahashi2025rest}.

%%%%%%%%%%%%%%%%%%%%%%%%%%%%%%%%%%%%%%%%%%%%%%%%%%%%%%%%%%%%%%%%%%%%%%%%%%%%%%%
%%%%%%%%%%%%%%%%%%%%%%%%%%%%%%%%%%%%%%%%%%%%%%%%%%%%%%%%%%%%%%%%%%%%%%%%%%%%%%%

\subsection{Stretching}
We define the stretching force of edge $i$ on vertex $i + 1$ as $\generalizedForce_{\mathrm{st, i, i + 1}} = -\nabla_{\vertexPos_{i+1}} E_{\mathrm{st, i}}(\vertexPos_{i}, \vertexPos_{i+1})$ \eqref{eq:stretch_grad}, and define $\generalizedForce_{\mathrm{st, i, i}}$ analogously. Given the dependence of $\generalizedForce_{\mathrm{st, i, i + 1}}$ and $\generalizedForce_{\mathrm{st, i, i}}$ on $\restLength_i$ and $\stretchCoef_i$, their Jacobians are
\begin{align}
\frac{\partial \generalizedForce_{\mathrm{st, i, i+1}}
}{\partial \restLength_i}
&= -
\frac{\partial \generalizedForce_{\mathrm{st, i, i}}
}{\partial \restLength_i}
= 
\stiffnessScale \stretchCoef_i \pi \radius^2 \length_i \restLength_i^{-2} \tangent_i,
\\
\frac{\partial \generalizedForce_{\mathrm{st, i, i+1}}
}{\partial \stretchCoef_i}
&= -
\frac{\partial \generalizedForce_{\mathrm{st, i, i}}
}{\partial \stretchCoef_i}
= 
- \stiffnessScale \pi \radius^2 \left(\length_i \restLength_i^{-1} - 1\right) \tangent_i.
\end{align}

%%%%%%%%%%%%%%%%%%%%%%%%%%%%%%%%%%%%%%%%%%%%%%%%%%%%%%%%%%%%%%%%%%%%%%%%%%%%%%%
%%%%%%%%%%%%%%%%%%%%%%%%%%%%%%%%%%%%%%%%%%%%%%%%%%%%%%%%%%%%%%%%%%%%%%%%%%%%%%%

\subsection{Bending}
We define the bending force according to \eqref{eq:bending_i_grad} by $\generalizedForce_{\mathrm{be}, i} = -\nabla E_{\mathrm{be}, i}(\yvec_i)$. Given its dependence on $\restLength_{i-1}, \restLength_{i}$, $\restCurvature_{i, 0}, \restCurvature_{i, 1}$, and $\bendCoef_i$ while respecting the constraints $\restCurvature_{i, 0} = \restCurvature_{i, 2}$ and $\restCurvature_{i, 1} = \restCurvature_{i, 3}$, the Jacobians are given (with $j \in \{0, 1\})$ by
\begin{align}
\frac{\partial \generalizedForce_{\mathrm{be}, i}}{\partial \restLength_{i-1}} &=
\frac{\partial \generalizedForce_{\mathrm{be}, i}}{\partial \restLength_{i}} = 
\left(\frac{\stiffnessScale \bendCoef_i \pi \radius^4}{4 (\restLength_{i-1} + \restLength_{i})^2}\right)
\mathbf{J}_{\mathrm{cu}, i}^T (\curvature_i - \restCurvature_i),
\\
\frac{\partial \generalizedForce_{\mathrm{be}, i}}{\partial \restCurvature_{i, j}} &=
\left(\frac{\stiffnessScale \bendCoef_i \pi \radius^4}{4 (\restLength_{i-1} + \restLength_{i})}\right)
(\nabla \curvature_{i, j} + \nabla \curvature_{i, j + 2}),
\\
\frac{\partial \generalizedForce_{\mathrm{be}, i}}{\partial \bendCoef_i} &= -
\left(\frac{\stiffnessScale \pi \radius^4}{4 (\restLength_{i-1} + \restLength_{i})}\right)
\mathbf{J}_{\mathrm{cu}, i}^T (\curvature_i - \restCurvature_i).
\end{align}

%%%%%%%%%%%%%%%%%%%%%%%%%%%%%%%%%%%%%%%%%%%%%%%%%%%%%%%%%%%%%%%%%%%%%%%%%%%%%%%
%%%%%%%%%%%%%%%%%%%%%%%%%%%%%%%%%%%%%%%%%%%%%%%%%%%%%%%%%%%%%%%%%%%%%%%%%%%%%%%

\subsection{Twisting}
We define the twisting force as $\generalizedForce_{\mathrm{tw}, i} = -\nabla E_{\mathrm{tw}, i}(\yvec_i)$ \eqref{eq:twist_i_grad}. Given its dependence on $\restLength_{i-1}, \restLength_{i}$, $\restTwist_{i}$, and $\twistCoef_i$, the Jacobians are given by
\begin{align}
\frac{\partial \generalizedForce_{\mathrm{tw}, i}}{\partial \restLength_{i-1}} &= \frac{\partial \generalizedForce_{\mathrm{tw}, i}}{\partial \restLength_{i}} =
\left(\frac{\stiffnessScale \twistCoef_i \pi \radius^4}{(\restLength_{i-1} + \restLength_{i})^2}\right)
(\twist_i - \restTwist_i) \nabla \twist_i,
\\
\frac{\partial \generalizedForce_{\mathrm{tw}, i}}{\partial \restTwist_{i}} &=
\left(\frac{\stiffnessScale \twistCoef_i \pi \radius^4}{(\restLength_{i-1} + \restLength_{i})}\right) \nabla \twist_i,
\\
\frac{\partial \generalizedForce_{\mathrm{tw}, i}}{\partial {\twistCoef}_{i}} &=-
\left(\frac{\stiffnessScale \pi \radius^4}{(\restLength_{i-1} + \restLength_{i})}\right)
(\twist_i - \restTwist_i) \nabla \twist_i.
\end{align}

%%%%%%%%%%%%%%%%%%%%%%%%%%%%%%%%%%%%%%%%%%%%%%%%%%%%%%%%%%%%%%%%%%%%%%%%%%%%%%%
%%%%%%%%%%%%%%%%%%%%%%%%%%%%%%%%%%%%%%%%%%%%%%%%%%%%%%%%%%%%%%%%%%%%%%%%%%%%%%%

\subsection{Bending With 2D vs. 4D Curvatures}
We begin by comparing bending formulations using 2D and 4D curvatures to justify our choice of 4D curvatures, given that our parameter optimization includes only two rest curvatures per vertex. The analysis is conducted on a horizontal strand discretized with 30 vertices.

%%%%%%%%%%%%%%%%%%%%%%%%%%%%%%%%%%%%%%%%%%%%%%%%%%%%%%%%%%%%%%%%%%%%%%%%%%%%%%%
%%%%%%%%%%%%%%%%%%%%%%%%%%%%%%%%%%%%%%%%%%%%%%%%%%%%%%%%%%%%%%%%%%%%%%%%%%%%%%%

\begin{figure} 
\centering
\subfloat[\label{1a}]{%
    \adjincludegraphics[trim={{0.1\width} {0.0\height} {0.2\width} {0.1\height}}, clip, width=0.25\linewidth]
    {figures/\figDir/bending_4vs2_2_angle0_0300.png}}
\subfloat[\label{1b}]{%
    \adjincludegraphics[trim={{0.1\width} {0.0\height} {0.2\width} {0.1\height}}, clip, width=0.25\linewidth]
    {figures/\figDir/bending_4vs2_2_angle180_0300.png}}
\subfloat[\label{1c}]{%
    \adjincludegraphics[trim={{0.1\width} {0.0\height} {0.2\width} {0.1\height}}, clip, width=0.25\linewidth]
    {figures/\figDir/bending_4vs2_4_angle0_0300.png}}
\subfloat[\label{1d}]{%
    \adjincludegraphics[trim={{0.1\width} {0.0\height} {0.2\width} {0.1\height}}, clip, width=0.25\linewidth]
    {figures/\figDir/bending_4vs2_4_angle180_0300.png}}
\caption{
Comparison of two bending models with a horizontal strand without and with flipped material frames. (a) 2D curvatures. (b) 2D curvatures with flipped frames. (c) 4D curvatures. (d) 4D curvatures with flipped frames. The bending model with 2D and 4D curvatures without frame flips can correctly evaluate bending and generate natural strand behaviors ((a) and (c)). With the flipped frames, the 2D curvature bending model fails to generate bending forces (b), whereas the 4D curvature bending model correctly handles the bending, generating the expected result (d).
}
\label{fig:bending_4vs2} 
\end{figure}

\subsubsection{2D Curvatures with Averaged Material Frames \cite{Bergou:2010:DVT:1778765.1778853}}
In Figure \ref{fig:bending_4vs2}, we compare a bending model with 4D curvatures \cite{Bergou2008} against a bending model with 2D curvatures \cite{Bergou:2010:DVT:1778765.1778853} which averages material frames to reduce curvature dimensions from 4D to 2D. We experiment with the horizontal strand without and with its material frames flipped, and use $\bendCoefFinal = 10^{10}$.

While both models without frame flips yield equivalent results, the 2D curvature model \cite{Bergou:2010:DVT:1778765.1778853} fails to generate bending forces when material frames are flipped because the averaged material frames can be non-unit vectors (in this example, averaged frames are zero vectors) \cite{Fei2019,Panetta2019,Gornowicz2015}. By contrast, the 4D curvature model \cite{Bergou2008} correctly evaluates the bending even with the flipped frames, producing results consistent with those obtained without edge flips.

%%%%%%%%%%%%%%%%%%%%%%%%%%%%%%%%%%%%%%%%%%%%%%%%%%%%%%%%%%%%%%%%%%%%%%%%%%%%%%%
%%%%%%%%%%%%%%%%%%%%%%%%%%%%%%%%%%%%%%%%%%%%%%%%%%%%%%%%%%%%%%%%%%%%%%%%%%%%%%%

\begin{figure} 
\centering
\subfloat[\label{1a}]{%
    \adjincludegraphics[trim={{0.0\width} {0.0\height} {0.5\width} {0.0\height}}, clip, width=0.25\linewidth]
    {figures/\figDir/slerp_slerp_1e8_0120.png}}
\subfloat[\label{1b}]{%
    \adjincludegraphics[trim={{0.0\width} {0.0\height} {0.5\width} {0.0\height}}, clip, width=0.25\linewidth]
    {figures/\figDir/slerp_slerp_1e9_0120.png}}
\subfloat[\label{1c}]{%
    \adjincludegraphics[trim={{0.0\width} {0.0\height} {0.5\width} {0.0\height}}, clip, width=0.25\linewidth]
    {figures/\figDir/slerp_curv4_1e8_0120.png}}
\subfloat[\label{1d}]{%
    \adjincludegraphics[trim={{0.0\width} {0.0\height} {0.5\width} {0.0\height}}, clip, width=0.25\linewidth]
    {figures/\figDir/slerp_curv4_1e9_0120.png}}
\caption{
Comparison of two bending models with a horizontal strand. 2D curvatures with slerp and $\bendCoefFinal = 10^8$ (a) and $\bendCoefFinal = 10^9$ (b). 4D curvatures with $\bendCoefFinal = 10^8$ (c) and $\bendCoefFinal = 10^9$ (d). While spherical interpolation enables correct evaluation of bending even with the flipped frames (b), approximated gradients can lead to stability problems (a). By contrast, the bending model with 4D curvatures generates natural strand behaviors ((c) and (d)).
}
\label{fig:slerp} 
\end{figure}

\subsubsection{2D Curvatures with Spherically Interpolated Material Frames \cite{Gornowicz2015}}
Figure \ref{fig:slerp} contrasts the bending model with 4D curvatures \cite{Bergou2008} against another model \cite{Gornowicz2015} with 2D curvatures, which spherically interpolates (i.e., uses slerp) material frames to maintain unit-size frames while reducing the curvature dimensions. We use flipped frames and $\bendCoefFinal = 10^8, 10^9$.

While the slerped material frames, which retain unit length, enable correct bending evaluation even with the flipped frames, differentiating the slerped frames to compute bending forces presents challenges. Consequently, their bending model \cite{Gornowicz2015} resorts to approximated gradients, which \mycolor{did not prove sufficiently accurate} in our experiments, causing stability problems with the Gauss-Newton Hessian approximation, whereas the bending model of \cite{Bergou2008} is stable under the same settings.
